# Supplementary material for: Dynamic locational marginal emissions via implicit differentiation
Source: arXiv:2302.14282 source file (2023-03-08)
Supplement: Supplementary file 1 [file Appendix.tex]

% \appendix


% \section{Modelling Assumptions}
% \label{apdx:models}

% \section{Experimental Details}
% \label{apdx:experiments}













\begin{comment}
\section{Computing sensitivities}

\paragraph{Computing sensitivities.} I will here try to lay out the details of the computation of the Jacobian and the implicit differentation scheme so that someone else can cross read and validate. 

First, let's write the optimization variables as 
$$
x = (x_1, x_2, ... x_T), \ x_t = (g_t, p_t, s_t). 
$$
Then, let's denote by $F$ and $H$ the matrices containing the inequality and equality constraints. We will decompose them in a similar way as above: 
$$
F = \begin{bmatrix}
F_1\\
F_2\\
\vdots\\
F_T
\end{bmatrix}, 
H = 
\begin{bmatrix}
H_1\\
H_2\\
\vdots\\
H_T
\end{bmatrix}. 
$$
All $F_t, H_t$ should have the same structure (with the exception of $H_0$ which needs to encode the initial condition for the nodal battery states of charge). For now, we will assume they all have the same form to get 95\% of the way there. 

We can there write an expression for both $F_t$ and $H_t$. We have
\begin{align*}
F_t^T &=
\begin{bmatrix}
-g_t, g_t - g_t^{\max}, -p_t-p_t^{\max}, p_t - p_t^{\max}, s_t - s_{t-1} - P, s_{t-1} - s_t - P, -s_t, s_t -C
\end{bmatrix},\\
H_t^T &=
\begin{bmatrix}
g_t - d_t - (s_t-s_{t-1}) - Ap_t
\end{bmatrix}.
\end{align*}
Once this is established, we can proceed to the expression of the KKT conditions in matrix form. The Lagrangian of the problem can be written as
\begin{align*}
    L = \sum_t\left( g_t^T \diag(c^q) g_t + g_t^T c^\ell + \lambda_t^T F_t + \nu_t^T H_t\right).
\end{align*}
Using the same notations as~\cite{Barratt2018OnProblems}, we want to first write the matrix
\begin{align*}
    g(z, \theta) = 
    \begin{bmatrix}
    \nabla_x L \\
    \diag(\lambda) F\\
    H
    \end{bmatrix}.
\end{align*}
The stationarity condition (i.e. the first block in the above matrix) yields: 
\begin{align*}
    \nabla_x L &= 
    \begin{bmatrix}
    \nabla_{x_1} L, ..., \nabla_{x_T} L
    \end{bmatrix}^T, \\
    \nabla_{x_t} L &= 
    \begin{bmatrix}
    \partial_{g_t} L\\
    \partial_{p_t} L \\
    \partial_{s_t} L\\
    \end{bmatrix}
    = 
    \begin{bmatrix}
    2\ \diag(c^q) g_t + c^\ell + \lambda_t^T D_{g_t}F_t + \nu_t^T D_{g_t}H_t \\
     \lambda_t^T D_{p_t}F_t + \nu_t^T D_{p_t}H_t\\
     \lambda_{t+1}^T D_{s_t} F_{t+1} + \lambda_t^T D_{s_t} F_{t} + \nu_{t+1}^T D_{s_t} H_{t+1} + \nu_t^T D_{s_t} H_t
    \end{bmatrix}.
\end{align*}
Therefore, the full computation of $\nabla_x L$ can be decomposed into suboperations at each timestep. However, it is not fully decomposable as can be seen in the last term of the above equation (there is coupling between subsequent timesteps. 

Now we proceed to the clear expression of the different Jacobians present in the above. 
For the inequality constraints we have
\begin{align*}
    D_{g_t} F_t =
    \begin{bmatrix}
    -I \\
    I \\
    0\\
    0\\
    0\\
    \vdots\\
    0
    \end{bmatrix}, 
    D_{p_t} F_t = 
    \begin{bmatrix}
    0 \\
    0 \\
    -I \\
    I\\
    0\\
    \vdots\\
    0
    \end{bmatrix}, 
    D_{s_t}F_t =
    \begin{bmatrix}
    0\\
    0\\
    0\\
    0\\
    I\\
    -I\\
    -I\\
    I
    \end{bmatrix}, 
    D_{s_t}F_{t+1} = 
    \begin{bmatrix}
    0\\
    0\\
    0\\
    0\\
    -I\\
    I\\
    0\\
    0
    \end{bmatrix}
\end{align*}

For the equality constraints we have
\begin{align*}
    D_{g_t} H_t = [I], D_{p_t}H_t = [-A], D_{s_t} H_t = [-I], D_{s_t}H_{t+1} = [I]
\end{align*}

All this detail will be useful when computing the complete Jacobian, which we proceed to do now. 
Again, borrowing notations from ~\cite{Barratt2018OnProblems} we want to compute
\begin{align*}
    D_z g = 
    \begin{bmatrix}
    D_x \nabla_x L & D_x F^T &  D_x H^T \\
    \diag(\lambda)D_xF & \diag(F) & 0 \\
    D_x H & 0 & 0
    \end{bmatrix}.
\end{align*}
We can easily decompose the jacobians in the expression above into the smaller timestep-level jacobians that we have computed above. 
Indeed
\begin{align*}
    D_xF = 
    \begin{bmatrix}
    D_{x_1} F_1 & ... & D_{x_T} F_1\\
    \vdots & ... & \vdots \\
    D_{x_1} F_T & ... & D_{x_T} F_T
    \end{bmatrix}
\end{align*}
and we have that
\begin{align*}
    D_{x_t} F_t =
    \begin{bmatrix}
    D_{g_t}F_t & D_{p_t}F_t & D_{s_t} F_t
    \end{bmatrix}
\end{align*}
and that
\begin{align*}
    D_{x_t} F_{t+1} = 
    \begin{bmatrix}
    0 & 0 &  D_{s_t} F_{t+1}
    \end{bmatrix}.
\end{align*}
Similarly, we have that
\begin{align*}
    D_{x_t}H_t = 
    \begin{bmatrix}
    I & -A & -I
    \end{bmatrix}, 
    D_{x_t} H_{t+1} = 
    \begin{bmatrix}
    0 & 0 & I
    \end{bmatrix}
\end{align*}
The above derivations should therefore be sufficient to compute the entire matrix $D_z g$. 

We have that
\begin{align*}
    D_x\nabla_x L = 
    \begin{bmatrix}
    D_{x_1} \nabla_{x_1} L & ... & D_{x_T} \nabla_{x_1} L \\
    \vdots & & \vdots \\ 
    D_{x_1} \nabla_{x_T} L & ... & D_{x_T} \nabla_{x_T} L \\
    \end{bmatrix}
\end{align*}

We have
\begin{align*}
    D_{x_i}\nabla_{x_j} L = \delta_{ij} 
    \begin{bmatrix}
    2 \diag(c^q) & 0 & 0 \\
    0 & 0 & 0 \\
    0 & 0 & 0
    \end{bmatrix}
\end{align*}

\paragraph{A note on computational burden.} With a graph of $N$ nodes and $E$ edges, we go from $N + E$ variables and $3(N+E)$ constraints to $2(NT)$ variables with ... constraints. The size of the matrix to invert (KKT) is ...? This limits the size of the time horizon to ...? 
Are there ways to leverage the structure of the matrix for easier inversion?
\end{comment}
